# Supplementary material for: Semi-supervised Learning with GANs: Manifold Invariance with Improved Inference
Source: arXiv:1705.08850 source file (2017-12-05)
Supplement: Supplementary file 1 [file appendix.tex]

\begin{center}{\Large \bf Appendix }\end{center}

\punt{
\section{Algorithm outline}

\begin{algorithm}[H]
		\KwData{Labeled examples $\{x_i,y_i\}_{i=1}^{N_l}$, unlabeled examples $\{x_i\}_{i=1}^{N_u}$}
	\begin{algorithmic}[1]

	\STATE \textbf{Train the Augmented-BiGAN} by optimizing the objective in Eq. \eqref{eq:augBigan} to learn the generator $g$, encoder $h$ and discriminator $f$. %      This gives an encoder $h(.)$ that maps data sample $x \in X$ to latent representation   $z \in Z$ as $z = h(x)$, a generator $g(.)$ that maps the latent representation back to    the data manifold as $x = g(z)$ and a discriminator $f(.)$ that maps the generated     image to $k+1$ classes.
	 \STATE \textbf{Estimate the dominant tangent directions} by learning a nonlinear (low-dimensional)      approximation in the $Z$-space such that $g(\bar{p}(p(h(x))))$ is close to $g(h(x))$, where     $p:R^d\to R^{d_p}$ and $\bar{p}:R^{d_p}\to R^d$ (with $d_p < d$). These are learned by optimizing      $\min_{p,\bar{p}} \mbb{E}_x [\lVert g(h(x))-g(\bar{p}(p(h(x))))\rVert_1 + \lVert f^{X}_{-1}(g(h(x))) - f^X_{-1}(g(\bar{p}(p(h(x)))))\rVert]$      while $g,h$ and $f$ are kept fixed from the pre-trained model. 
	%    Discriminator $f$ has two pipelines $f^Z$ and $f^X$ for the latent $z$ and the data $x$, \\      respectively, which share parameters in the last few layers, and the last layer of $f^X$ is used in this loss.  \\
	    Use the Jacobian of $p\circ h$, $J_x\, p\circ h$, as an estimate of the $d_p$ dominant tangent directions. 
	\STATE   - \textbf{Train Classifier using TangentProp}: Apart form the regular classification loss,      add the following terms based on stoachistoc approximation of Jacobians: 
	     $\lVert c(x_i+v) - c(x_i)\rVert_2^2$ with $v$ randomly sampled (i.i.d.) from the set of tangents $T_{x_i}$,
	    and $\lVert c(x+\delta) - c(x)\rVert_2^2$ with $\delta\sim N(0,\sigma^2 I)$ (i.i.d), to achieve invariance in tangent      directions and small random perturbations, respectively.
		\end{algorithmic}
	\caption{Outline of the proposed Semi-supervised learning framework.}
\end{algorithm}

\begin{table}[h]
	\centering
	\caption{Outline of the proposed Semi-supervised learning framework.}
	\begin{tabular}{|l|}
		\hline
		\textbf{Input} \\
		- Data matrix, $X \in \mbb{R}^{N \times D}$  \\
		- Class labels, $Y \in \mbb{R}^{N \times k}$ \\ \\
		\textbf{Algorithm}\\
		\quad - \textbf{Train the Augmented-BiGAN}: that optimizes the objective in equation \ref{eq:augBigan}. \\ \quad \quad  This gives an encoder $h(.)$ that maps data sample $x \in X$ to latent representation \\ \quad \quad $z \in Z$ as $z = h(x)$, a generator $g(.)$ that maps the latent representation back to \\ \quad \quad the data manifold as $x = g(z)$ and a discriminator $f(.)$ that maps the generated \\ \quad \quad image to $k+1$ classes.\\
		\quad - \textbf{Obtain the dominant tangent directions}: by learning a nonlinear (low-dimensional) \\ \quad \quad approximation in the $Z$ space such that $g(\bar{p}(p(h(x))))$ is close to $g(h(x))$, where \\ \quad \quad $p:R^d\to R^{d_p}$ and $\bar{p}:R^{d_p}\to R^d$ (with $d_p < d$). These are learned by optimizing \\ \quad \quad  $\min_{p,\bar{p}} \mbb{E}_x [\lVert g(h(x))-g(\bar{p}(p(h(x))))\rVert_1 + \lVert f^{X}_{-1}(g(h(x))) - f^X_{-1}(g(\bar{p}(p(h(x)))))\rVert]$ \\ \quad \quad while $g,h$ and $f$ are kept fixed from the pre-trained model. \\ 
		%\quad \quad Discriminator $f$ has two pipelines $f^Z$ and $f^X$ for the latent $z$ and the data $x$, \\ \quad \quad  respectively, which share parameters in the last few layers, and the last layer of $f^X$ is used in this loss.  \\
		\quad \quad Use the Jacobian of $p\circ h$, $J_x\, p\circ h$, as an estimate of the $d_p$ dominant tangent directions. \\
		\quad - \textbf{Train Classifier using TangentProp}: Apart form the regular classification loss, \\ \quad \quad add the following terms based on stoachistoc approximation of Jacobians: \\
		\quad \quad  $\lVert c(x_i+v) - c(x_i)\rVert_2^2$ with $v$ randomly sampled (i.i.d.) from the set of tangents $T_{x_i}$,\\ 
		\quad \quad and $\lVert c(x+\delta) - c(x)\rVert_2^2$ with $\delta\sim N(0,\sigma^2 I)$ (i.i.d), to achieve invariance in tangent \\ \quad \quad directions and small random perturbations, respectively.\\
		\hline
	\end{tabular}
	\label{Table:algorithm}
\end{table}
}

%\newpage
\section{Tangent Plots}

\begin{figure}[!h]
	\centering
    \includegraphics[width=\textwidth]{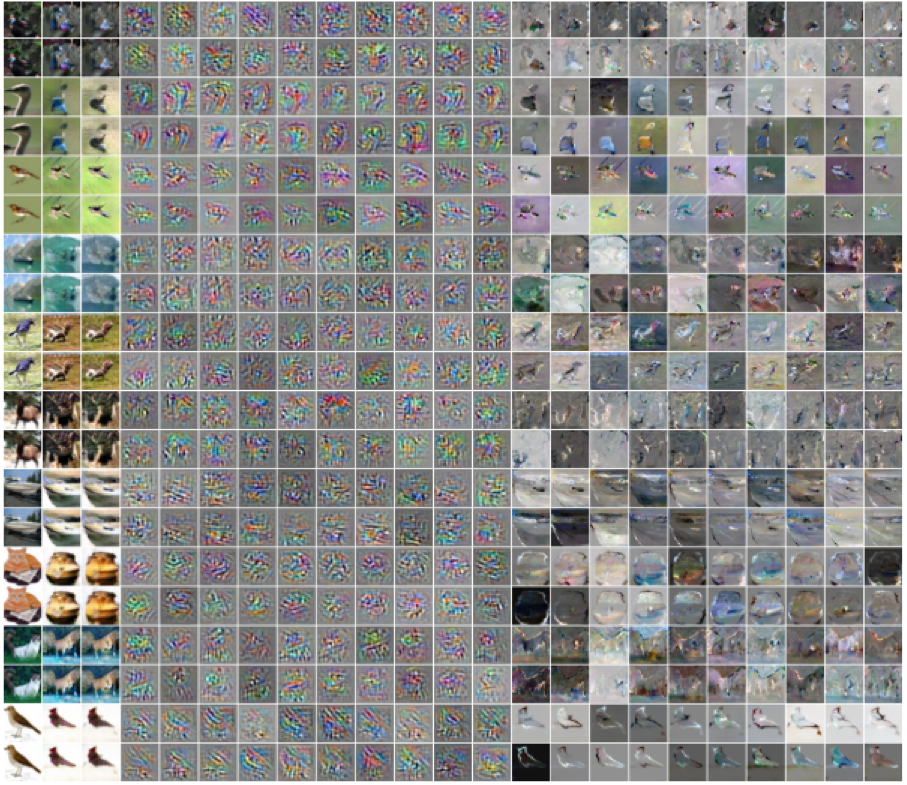}
    \caption{CIFAR10 tangents. \emph{Odd rows:} Tangents using our method for estimating the dominant tangent space. \emph{Even rows:} Tangents using SVD on $J_{h(x)} g$ and $J_x h$. \emph{First column:} Original image. \emph{Second column:} Reconstructed image using $g \circ h$. \emph{Third column:} Reconstructed image using $g\circ \bar{p} \circ p \circ h$. \emph{Columns 4-13:} Tangents using encoder. \emph{Columns 14-23:} Tangents using generator.}
\end{figure}
    
\begin{figure}[!h]
	\centering
    \includegraphics[width=\textwidth]{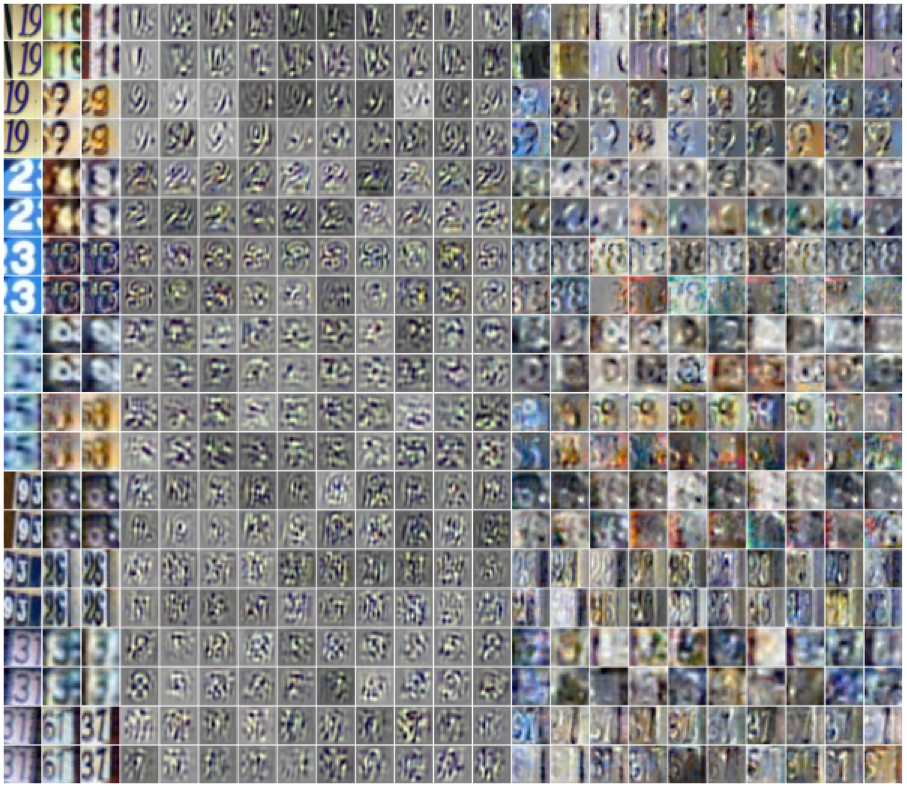}
    \caption{SVHN tangents. \emph{Odd rows:} Tangents using our method for estimating the dominant tangent space. \emph{Even rows:} Tangents using SVD on $J_{h(x)} g$ and $J_x h$. \emph{First column:} Original image. \emph{Second column:} Reconstructed image using $g \circ h$. \emph{Third column:} Reconstructed image using $g\circ \bar{p} \circ p \circ h$. \emph{Columns 4-13:} Tangents using encoder. \emph{Columns 14-23:} Tangents using generator.}

\end{figure}

\newpage

\section{Reconstruction Plots}

\begin{figure}[h]
	\centering
    \includegraphics[width=\textwidth]{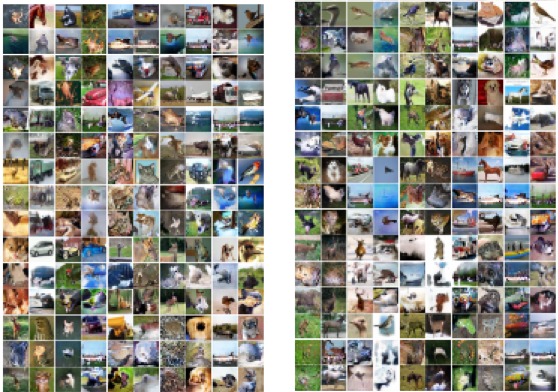}
    \caption{CIFAR10 reconstructions: Comparing BiGAN reconstructions with Augmented-BiGAN reconstructions. For $i=0,1,\ldots,4$, $(3i+1)$th row shows the original images, followed by BiGAN reconstructions in the $(3i+2)$'th row, and the Augmented-BiGAN reconstructions in the $(3i+3)$'th row. Reconstructions shown for total $100$ randomly sampled images from the test set ($10\times 5=50$ images each in the left and right column) from the test set.}
\end{figure}
    
\begin{figure}[h]
	\centering
    \includegraphics[width=\textwidth]{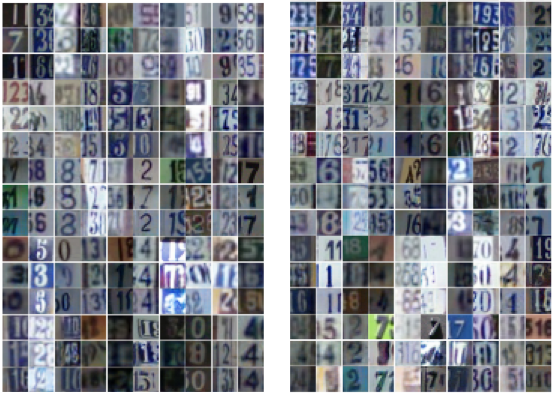}
    \caption{SVHN reconstructions: Comparing BiGAN reconstructions with Augmented-BiGAN reconstructions. For $i=0,1,\ldots,4$, $(3i+1)$th row shows the original images, followed by BiGAN reconstructions in the $(3i+2)$'th row, and the Augmented-BiGAN reconstructions in the $(3i+3)$'th row. Reconstructions shown for total $100$ randomly sampled images from the test set ($10\times 5=50$ images each in the left and right column).}
\end{figure}
